# Supplementary material for: ELDA: Using Edges to Have an Edge on Semantic Segmentation Based UDA
Source: arXiv:2211.08888 source file (2022-11-16)
Supplement: Supplementary file 1 [file all.tex]

% \section{Reproducibility}
% \label{sec::notation}
% \input{supplementary/reproducibility.tex}

\section{Notation Table}
\label{sec::notation}

The symbols used in this paper are summarized in Table~\ref{tab:supp:notation}.

\begin{table*}[tp]

\newcommand{\mytoprule}{\toprule[1.2pt]}
\centering
\setlength{\tabcolsep}{1.5em}
\footnotesize
\resizebox{.9\linewidth}{!}{%
\begin{tabularx}{\linewidth}{c|l}
\mytoprule
    Symbol & Description  \\
    \mytoprule
    $\Xs$ & A set of training images from the source domain. \\
    $\Xt$ & A set of training images from the target domain. \\
    $\Ys$ & The set of ground truth semantic segmentation labels \\& corresponding to $\Xs$.\\
    \hline
    $\xs$ & An image from the source domain. \\
    $\ys$ & The ground truth semantic segmentation label corresponding to $\xs$. \\
    $\C(\xs)$ & The edges generated by the Canny algorithm from $\xs$. \\
    $\xt$ & An image from the target domain. \\
    $\ypt$ & The pseudo semantic segmentation label corresponding to $\xt$. \\
    $\C(\xt)$ & The edges generated by the Canny algorithm from $\xt$. \\
    \hline
    $\C(\cdot)$ & The Canny operator. \\
    \hline
    $\yshatinit$ & The initial semantic segmentation prediction for $\xs$. \\
    $\ythatinit$ & The initial semantic segmentation prediction for $\xt$. \\
    $\yshatfinal$ & The final semantic segmentation prediction for $\xs$. \\
    $\ythatfinal$ & The final semantic segmentation prediction for $\xt$. \\
    $\eshatinit$ & The initial edge prediction for $\xs$. \\
    $\ethatinit$ & The initial edge prediction for $\xt$. \\
    $\eshatfinal$ & The final edge prediction for $\xs$. \\
    $\ethatfinal$ & The final edge prediction for $\xt$. \\
    $\lambda$ & A balancing factor for the segmentation and edge prediction tasks.\\
    \mytoprule
\end{tabularx}}
\caption{A list of the symbols used in this paper.}
\label{tab:supp:notation}
\end{table*}

% \vspace*{3cm}

% \clearpage

\section{Datasets}
\label{sec::datasets}
In this section, we describe the details of the datasets used in the experiments of this paper.

\subsection{Cityscapes Dataset}
The Cityscapes dataset~\cite{cordts2016cityscapes} is a real-world dataset containing semantic segmentation of a number of urban scenes. We use $2,975$ unlabeled images for training and 500 images for validation. The resolution is set to $2048 \times 1024$ pixels.

\subsection{GTA5 Dataset}
The GTA5 dataset~\cite{richter2016playing} is a synthetic dataset. It contains $24,966$ images with the resolution set to $1914 \times 1052$ pixels.  The images are labeled with Cityscapes-style annotations that include $19$ classes. In our experiments, we use the entire dataset as our source domain samples for training ELDA as well as the baselines.

\subsection{SYNTHIA Dataset}
The SYNTHIA dataset~\cite{Ros_2016_CVPR} is a synthetic dataset that is generated from an autonomous driving simulator of a number of urban scenes. 
% As an usual setup, 
In our experiments, we use the SYNTHIA-RAND-CITYSCAPES subset, which contains 9,400 images with the resolution set to $1280 \times 760$ pixels.  The images are labeled with Cityscapes-style annotations of $16$ classes.

\section{Implementation Details}
\label{sec::implementation details}
In this section, we elaborate on the implementation details of ELDA. We adopt Deeplabv2\cite{chen2017deeplab} with ResNet-101\cite{he2015deep} as the backbone of ELDA. Our model is trained using the SGD optimizer~\cite{DBLP:journals/corr/Ruder16} with a learning rate $2.5\times10^{-4}$ decayed by a factor of $0.9$ for $250,000$ iterations. The weight decay of the model parameters is set to $5\times10^{-4}$, and the momentum is set to 0.9. Images are randomly cropped to $512 \times 512$ pixels. The balancing factor $\lambda$ is set as $0.01$ and $1$ for GTA5$\to$Cityscapes and SYNTHIA$\to$Cityscapes benchmarks, respectively. The hyper-parameter $\sigma$ for the Canny operator is set to $2$. The batch size is set to $4$, where in each mini-batch there are two images from $\Xs$ and two images from $\Xt$. The code is implemented using Python with the PyTorch library~\cite{NEURIPS2019_9015}. All the methods are trained and evaluated on an NVIDIA Tesla V100 GPU.

\section{Visualization of Additional Qualitative Results}
\label{sec::visualization}

In this section, we present additional qualitative results, including the semantic segmentation predictions from \textit{source only}, CorDA~\cite{wang2021domain}, and ELDA in Fig.~\ref{fig:Seg_Qualitative_Result}, as well as the edge predictions from ELDA and the Canny algorithm in Fig.~\ref{fig:Edge_Qualitative_Result}.

\begin{figure}[tp]
  \centering
  \includegraphics[width=\linewidth]{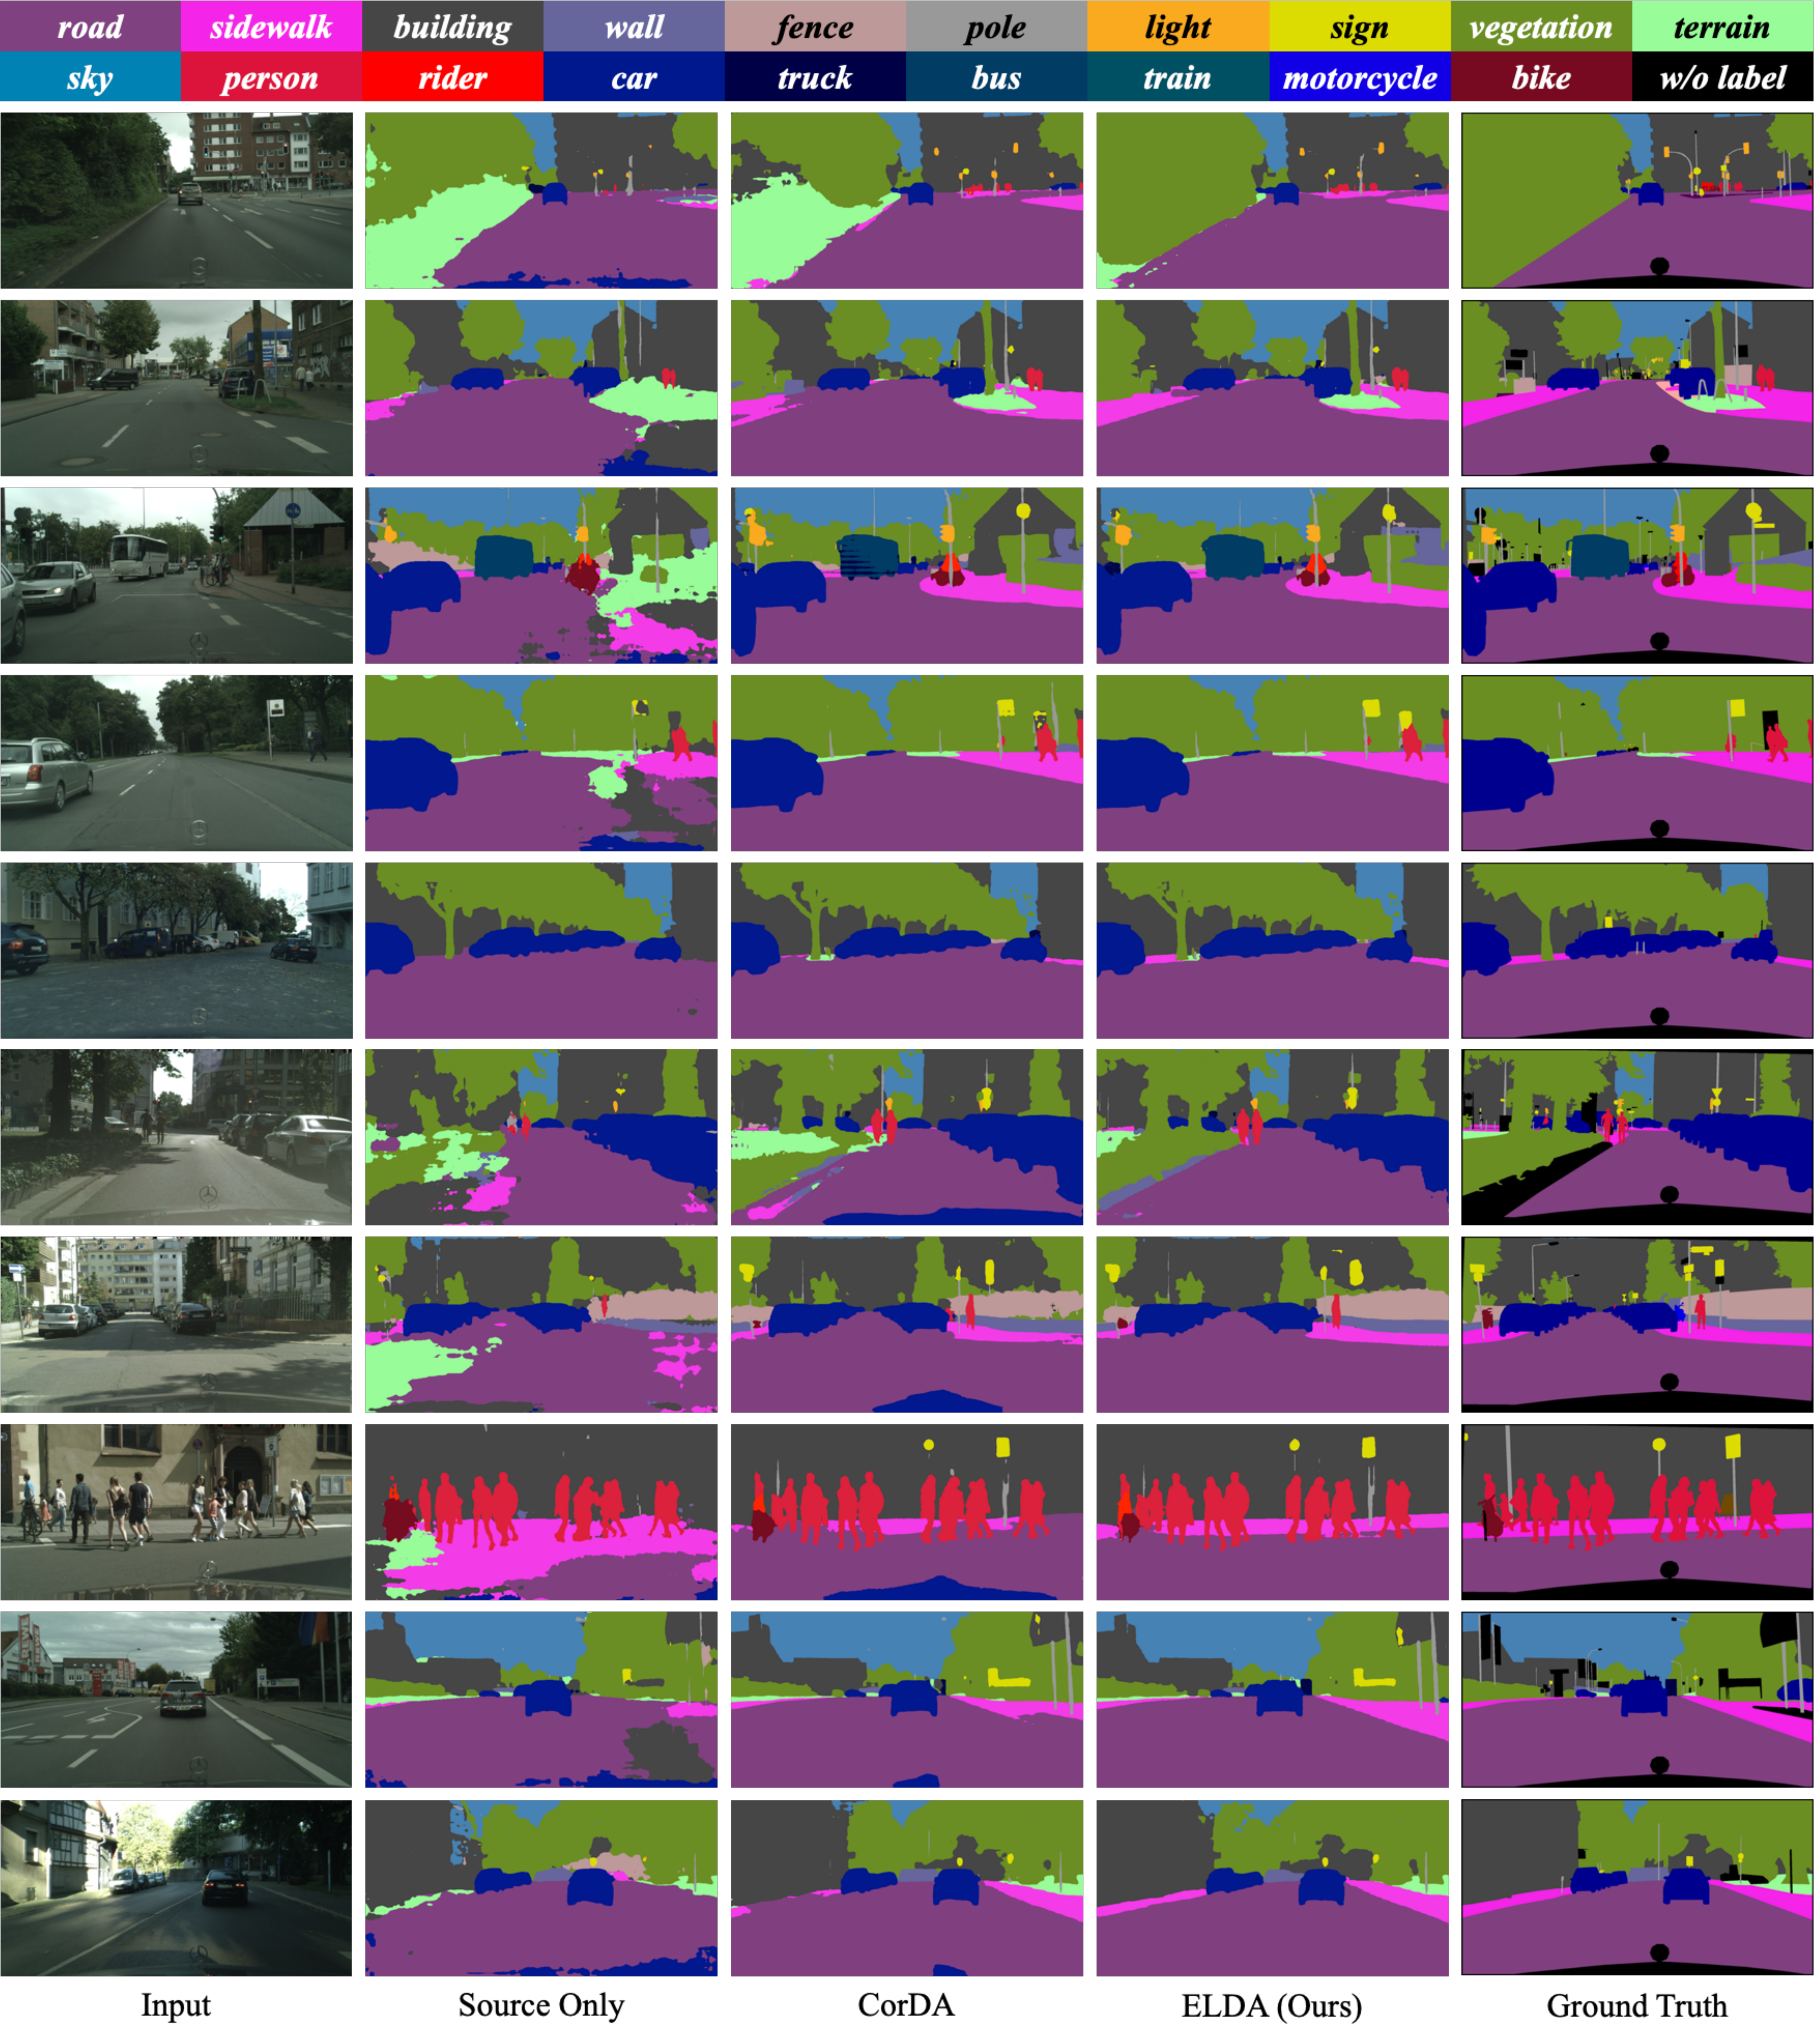}
  \caption{An illustration of the semantic segmentation predictions from \textit{source only}, CorDA~\cite{wang2021domain}, and ELDA, along with their corresponding input images and the ground truths. It can be observed that the predictions from ELDA are less noisy, and are able to preserve the boundaries in the predicted segmentation maps better than the other two baseline approaches.
  }
  \label{fig:Seg_Qualitative_Result}
\end{figure}

\begin{figure}[tp]
  \centering
  \includegraphics[width=.7\linewidth]{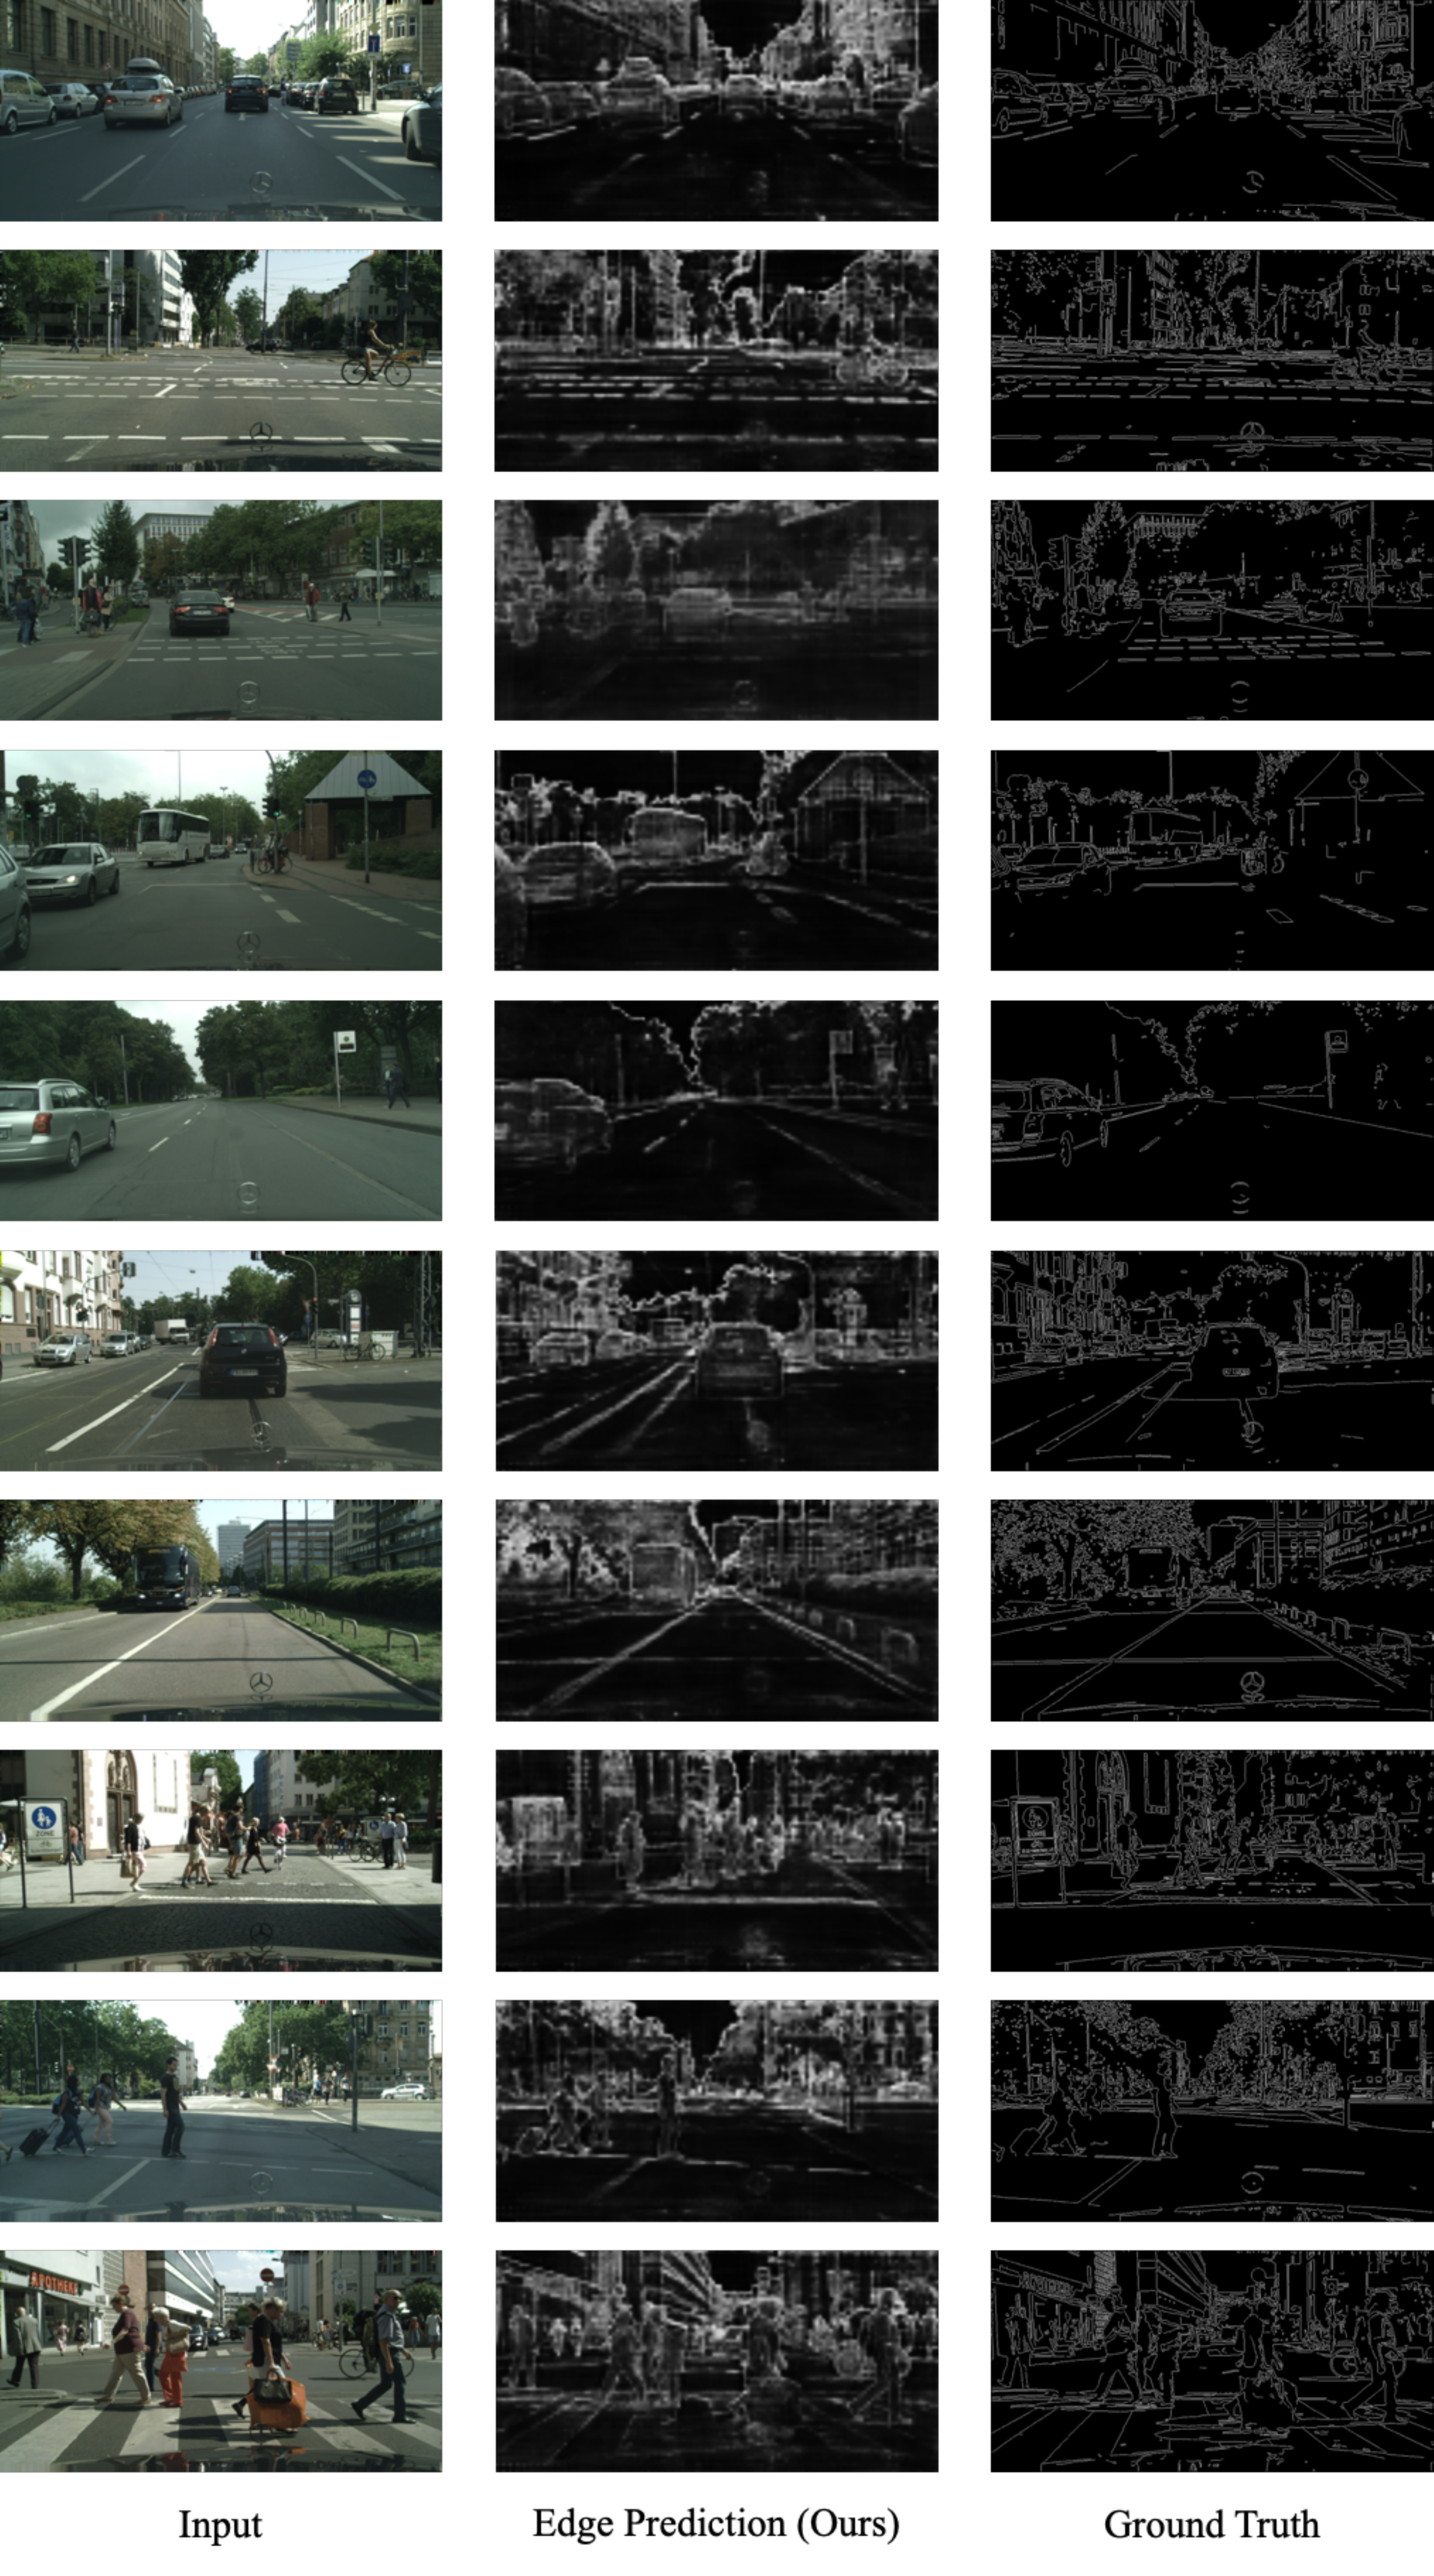}
  \caption{A comparison of the edge predictions from ELDA and the Canny algorithm. It can be observed that the edges predicted by ELDA are close to those generated by the Canny algorithm, indicating that ELDA is able to capture the essential edge features from its input images.}
  \label{fig:Edge_Qualitative_Result}
\end{figure}

% \section{Canny algorithm}
% \label{sec::canny}
% \input{supplementary/canny.tex}

% \section{Experimental Results}
% \label{sec::experiments}
% \input{sections/experiments.tex}

% \section{Conclusions}
% \label{sec::conclusions}
% \input{sections/conclusions.tex}
