# Supplementary material for: ELDA: Using Edges to Have an Edge on Semantic Segmentation Based UDA
Source: arXiv:2211.08888 source file (2022-11-16)
Supplement: Supplementary file 2 [file canny.tex]

% Edge可以透過canny algorithm [cite] 來獲得，演算法中主要分為 4 步驟：(1) 會先使用 Gaussian filer 來濾除 image 中的雜訊，其中可以控制 Gaussian filer 中sigma 值(後面記作 \sigma)的大小，當sigma 值越大濾掉越多雜訊 ，(2) 透過 sobel kernel [cite] 找出 pixel-wise gradient 的方向以及大小 (3) 藉由pixel-wise gradient 的方向以及大小判斷是否為local maximum，而 local maximum 是判定是否存在edge 的依據，(4) 最後透過 thresholding 來確認最終的edge。我們將以上的步驟定義為canny operator C(\cdot).
