# Supplementary material for: ELDA: Using Edges to Have an Edge on Semantic Segmentation Based UDA
Source: arXiv:2211.08888 source file (2022-11-16)
Supplement: Supplementary file 3 [file datasets.tex]

In this section, we describe the details of the datasets used in the experiments of this paper.

\subsection{Cityscapes Dataset}
The Cityscapes dataset~\cite{cordts2016cityscapes} is a real-world dataset containing semantic segmentation of a number of urban scenes. We use $2,975$ unlabeled images for training and 500 images for validation. The resolution is set to $2048 \times 1024$ pixels.

\subsection{GTA5 Dataset}
The GTA5 dataset~\cite{richter2016playing} is a synthetic dataset. It contains $24,966$ images with the resolution set to $1914 \times 1052$ pixels.  The images are labeled with Cityscapes-style annotations that include $19$ classes. In our experiments, we use the entire dataset as our source domain samples for training ELDA as well as the baselines.

\subsection{SYNTHIA Dataset}
The SYNTHIA dataset~\cite{Ros_2016_CVPR} is a synthetic dataset that is generated from an autonomous driving simulator of a number of urban scenes. 
% As an usual setup, 
In our experiments, we use the SYNTHIA-RAND-CITYSCAPES subset, which contains 9,400 images with the resolution set to $1280 \times 760$ pixels.  The images are labeled with Cityscapes-style annotations of $16$ classes.
