# Supplementary material for: ELDA: Using Edges to Have an Edge on Semantic Segmentation Based UDA
Source: arXiv:2211.08888 source file (2022-11-16)
Supplement: Supplementary file 4 [file implementation.tex]

In this section, we elaborate on the implementation details of ELDA. We adopt Deeplabv2\cite{chen2017deeplab} with ResNet-101\cite{he2015deep} as the backbone of ELDA. Our model is trained using the SGD optimizer~\cite{DBLP:journals/corr/Ruder16} with a learning rate $2.5\times10^{-4}$ decayed by a factor of $0.9$ for $250,000$ iterations. The weight decay of the model parameters is set to $5\times10^{-4}$, and the momentum is set to 0.9. Images are randomly cropped to $512 \times 512$ pixels. The balancing factor $\lambda$ is set as $0.01$ and $1$ for GTA5$\to$Cityscapes and SYNTHIA$\to$Cityscapes benchmarks, respectively. The hyper-parameter $\sigma$ for the Canny operator is set to $2$. The batch size is set to $4$, where in each mini-batch there are two images from $\Xs$ and two images from $\Xt$. The code is implemented using Python with the PyTorch library~\cite{NEURIPS2019_9015}. All the methods are trained and evaluated on an NVIDIA Tesla V100 GPU.
