# Supplementary material for: ELDA: Using Edges to Have an Edge on Semantic Segmentation Based UDA
Source: arXiv:2211.08888 source file (2022-11-16)
Supplement: Supplementary file 5 [file notation.tex]

The symbols used in this paper are summarized in Table~\ref{tab:supp:notation}.

\begin{table*}[tp]

\newcommand{\mytoprule}{\toprule[1.2pt]}
\centering
\setlength{\tabcolsep}{1.5em}
\footnotesize
\resizebox{.9\linewidth}{!}{%
\begin{tabularx}{\linewidth}{c|l}
\mytoprule
    Symbol & Description  \\
    \mytoprule
    $\Xs$ & A set of training images from the source domain. \\
    $\Xt$ & A set of training images from the target domain. \\
    $\Ys$ & The set of ground truth semantic segmentation labels \\& corresponding to $\Xs$.\\
    \hline
    $\xs$ & An image from the source domain. \\
    $\ys$ & The ground truth semantic segmentation label corresponding to $\xs$. \\
    $\C(\xs)$ & The edges generated by the Canny algorithm from $\xs$. \\
    $\xt$ & An image from the target domain. \\
    $\ypt$ & The pseudo semantic segmentation label corresponding to $\xt$. \\
    $\C(\xt)$ & The edges generated by the Canny algorithm from $\xt$. \\
    \hline
    $\C(\cdot)$ & The Canny operator. \\
    \hline
    $\yshatinit$ & The initial semantic segmentation prediction for $\xs$. \\
    $\ythatinit$ & The initial semantic segmentation prediction for $\xt$. \\
    $\yshatfinal$ & The final semantic segmentation prediction for $\xs$. \\
    $\ythatfinal$ & The final semantic segmentation prediction for $\xt$. \\
    $\eshatinit$ & The initial edge prediction for $\xs$. \\
    $\ethatinit$ & The initial edge prediction for $\xt$. \\
    $\eshatfinal$ & The final edge prediction for $\xs$. \\
    $\ethatfinal$ & The final edge prediction for $\xt$. \\
    $\lambda$ & A balancing factor for the segmentation and edge prediction tasks.\\
    \mytoprule
\end{tabularx}}
\caption{A list of the symbols used in this paper.}
\label{tab:supp:notation}
\end{table*}

% \vspace*{3cm}
