# Supplementary material for: ELDA: Using Edges to Have an Edge on Semantic Segmentation Based UDA
Source: arXiv:2211.08888 source file (2022-11-16)
Supplement: Supplementary file 6 [file reproducibility.tex]

Our code is available at
\url{https://anonymous.4open.science/r/ELDA-6738}.  All the experimental results presented in this paper are fully reproducible and verifiable.
