# Supplementary material for: ELDA: Using Edges to Have an Edge on Semantic Segmentation Based UDA
Source: arXiv:2211.08888 source file (2022-11-16)
Supplement: Supplementary file 7 [file visualization.tex]

In this section, we present additional qualitative results, including the semantic segmentation predictions from \textit{source only}, CorDA~\cite{wang2021domain}, and ELDA in Fig.~\ref{fig:Seg_Qualitative_Result}, as well as the edge predictions from ELDA and the Canny algorithm in Fig.~\ref{fig:Edge_Qualitative_Result}.

\begin{figure}[tp]
  \centering
  \includegraphics[width=\linewidth]{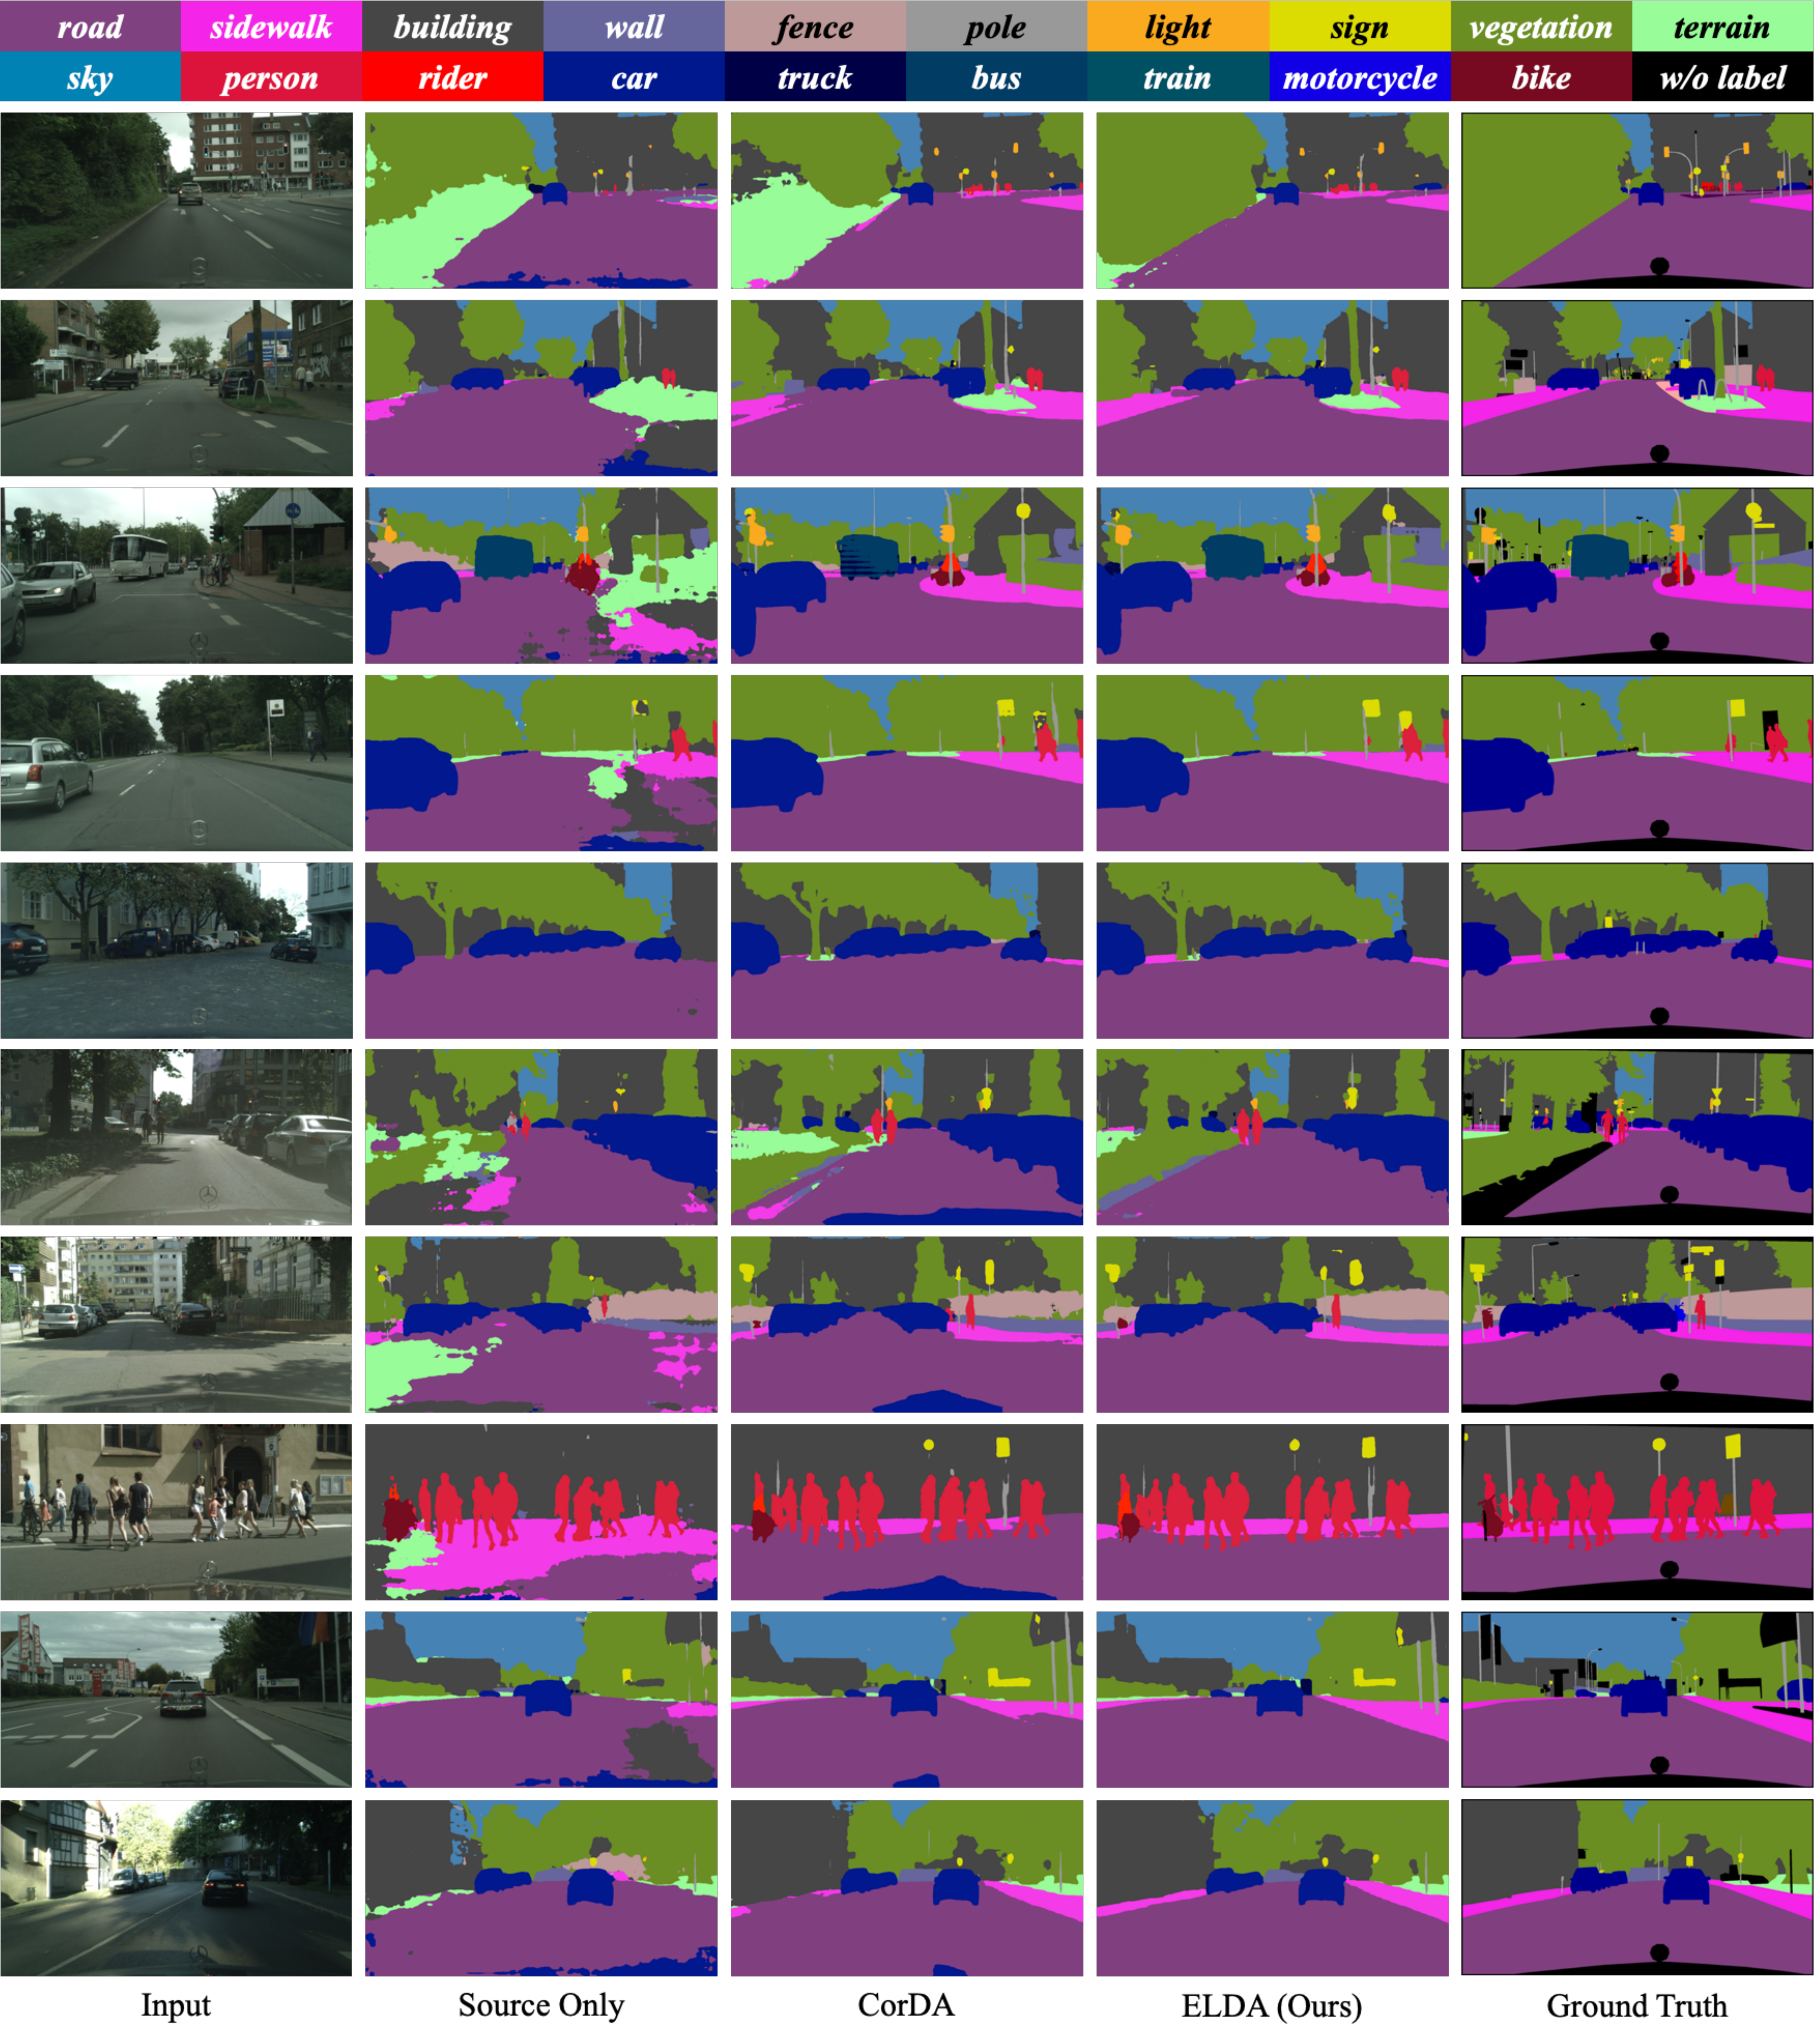}
  \caption{An illustration of the semantic segmentation predictions from \textit{source only}, CorDA~\cite{wang2021domain}, and ELDA, along with their corresponding input images and the ground truths. It can be observed that the predictions from ELDA are less noisy, and are able to preserve the boundaries in the predicted segmentation maps better than the other two baseline approaches.
  }
  \label{fig:Seg_Qualitative_Result}
\end{figure}

\begin{figure}[tp]
  \centering
  \includegraphics[width=.7\linewidth]{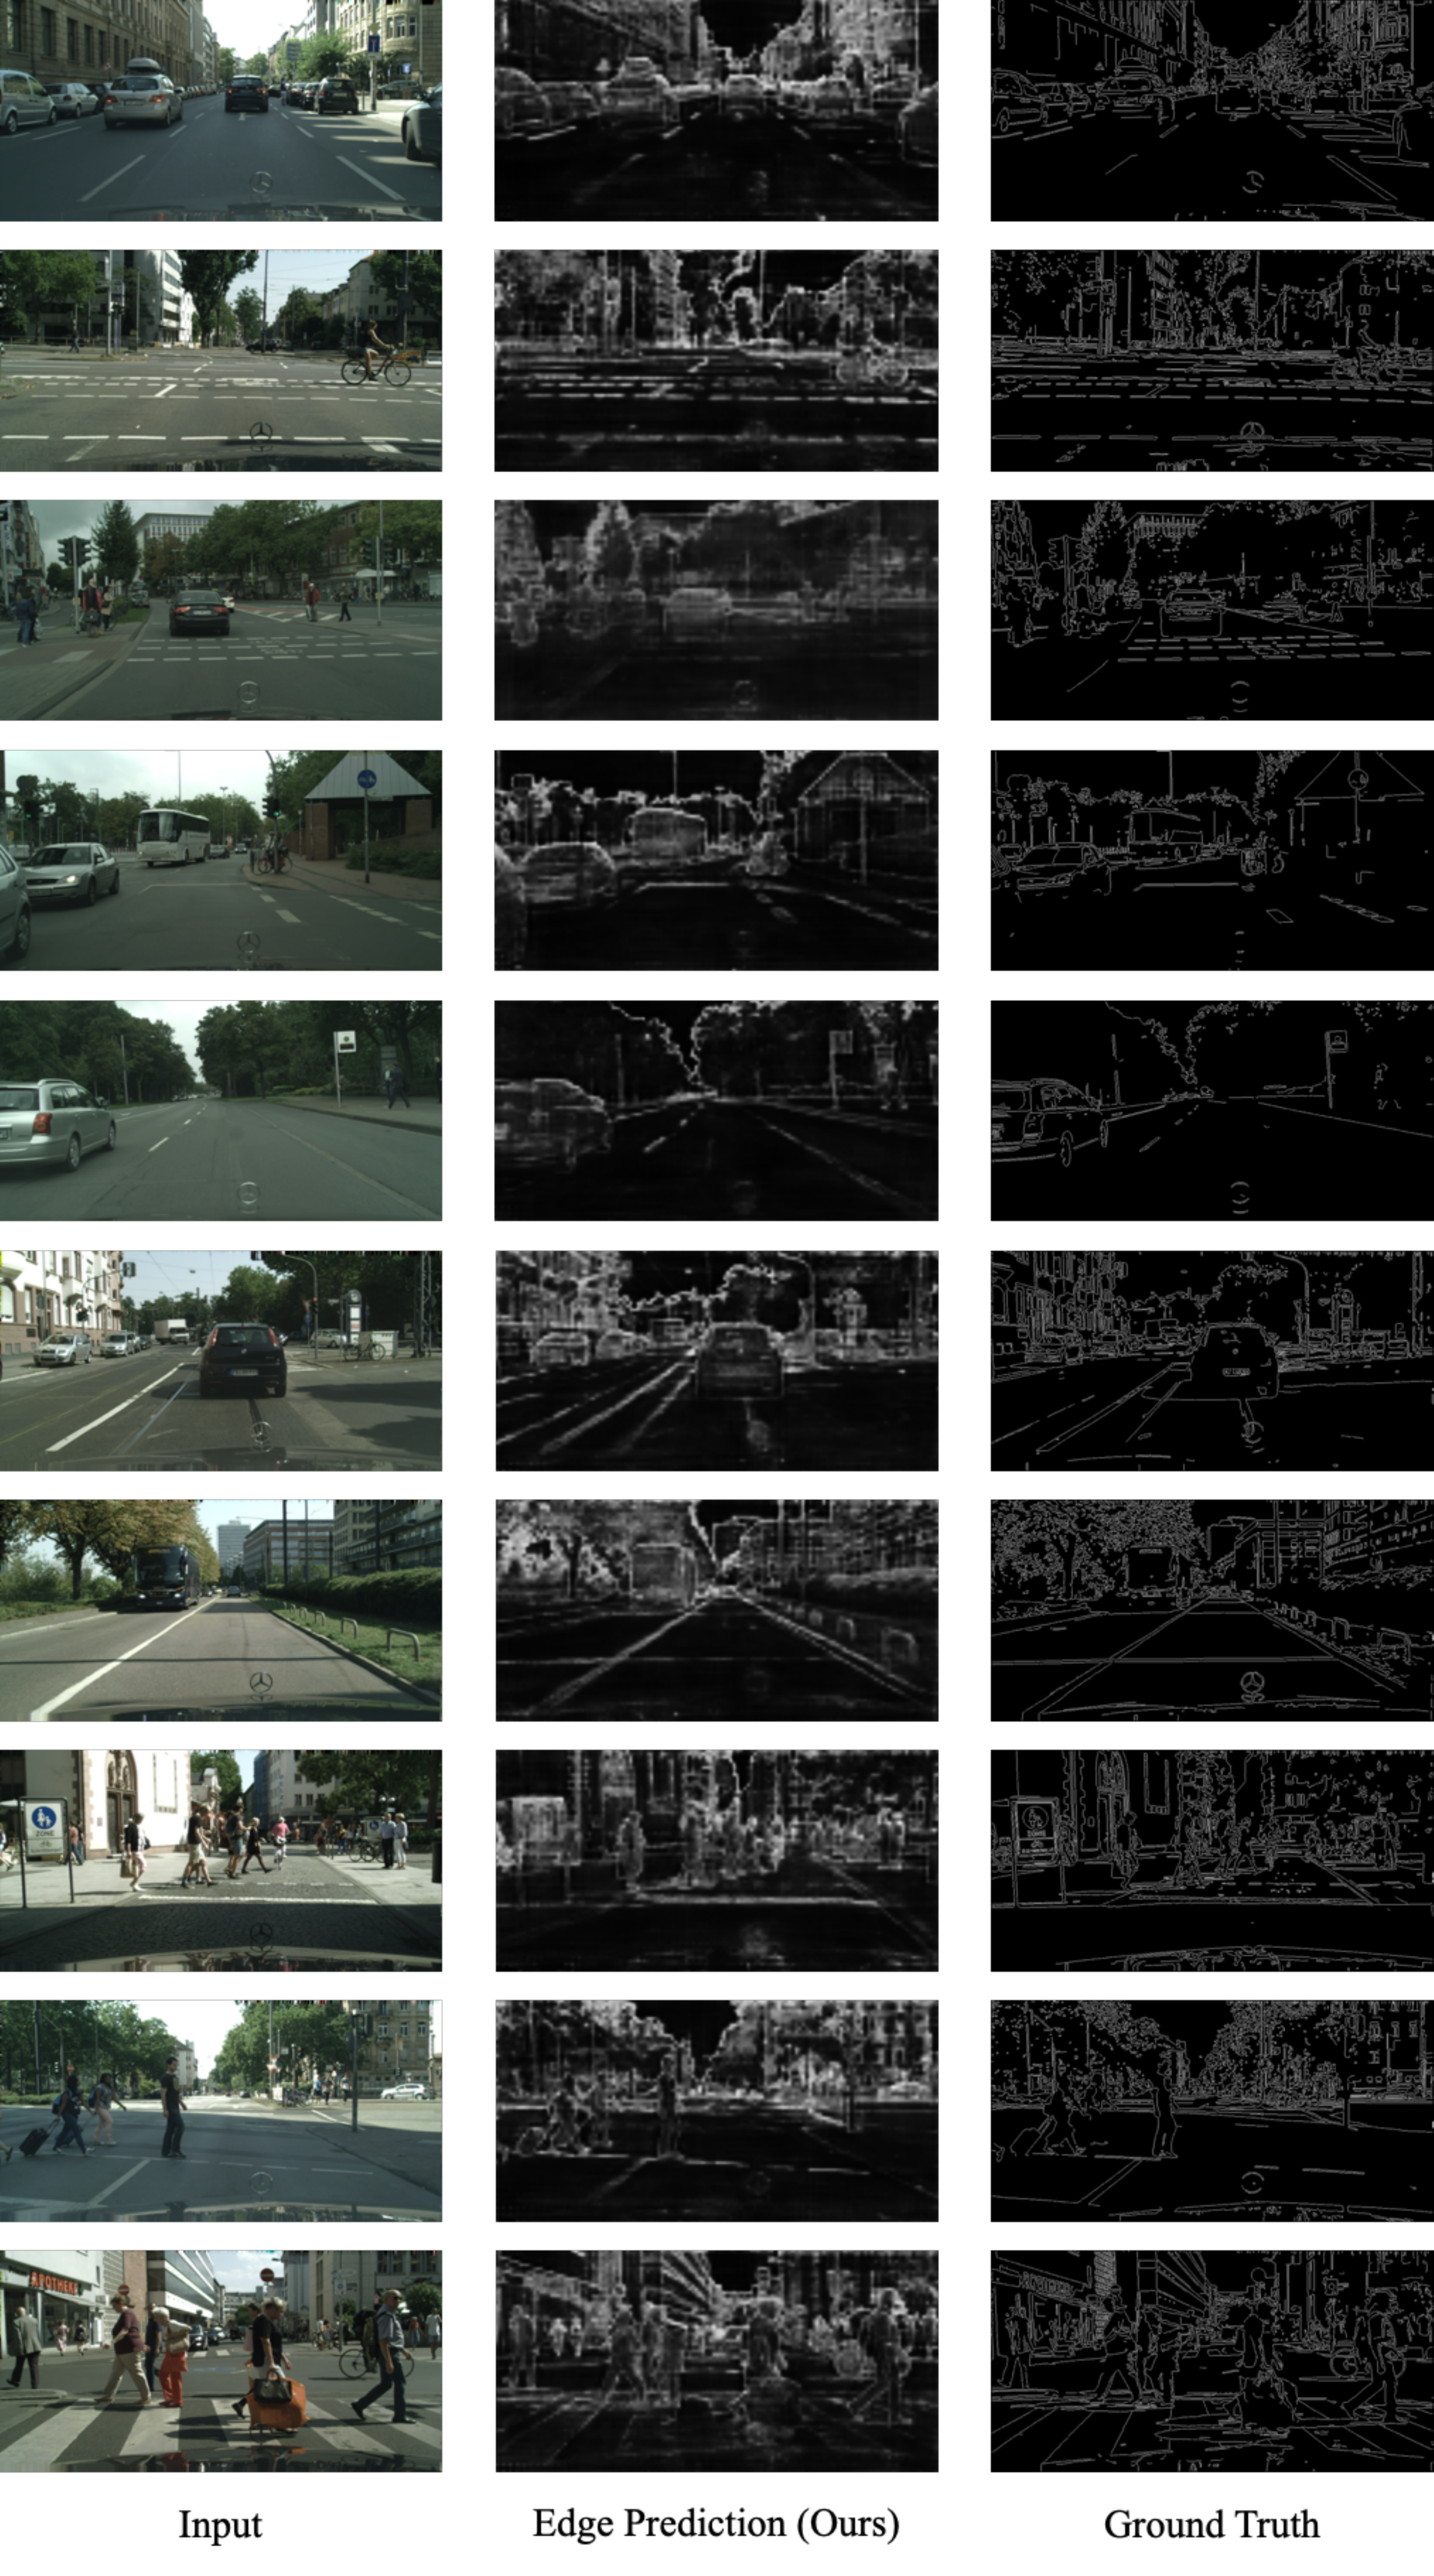}
  \caption{A comparison of the edge predictions from ELDA and the Canny algorithm. It can be observed that the edges predicted by ELDA are close to those generated by the Canny algorithm, indicating that ELDA is able to capture the essential edge features from its input images.}
  \label{fig:Edge_Qualitative_Result}
\end{figure}
